# Supplementary material for: Thermal and electrical cross-plane conductivity at the nanoscale in poly(3,4-ethylenedioxythiophene):trifuoromethanesulfonate thin films
Source: arXiv:2203.13326 source file (2022-03-24)
Supplement: Supplementary file 1 [file Supplementary_Data_PEDOT_nanoscale_transport.pdf]

# Supplementary Materials

## **Thermal and electrical cross-plane conductivity in poly(3,4-ethylenedioxythiophene): trifluoromethanesulfonate thin films**

K. Kondratenko\*, D. Guerin, X. Wallart, S. Lenfant and D. Vuillaume \*

*Institut d'Electronique Microélectronique et Nanotechnologie (IEMN), CNRS, Villeneuve  
d'Ascq, France*

\* Corresponding authors: [kirill.kondratenko@iemn.fr](mailto:kirill.kondratenko@iemn.fr), [dominique.vuillaume@iemn.fr](mailto:dominique.vuillaume@iemn.fr)

## 1. Preparation of PEDOT:OTf thin films

PEDOT:OTf thin films were prepared by spin-coating a precursor solution containing 3,4-ethylenedioxythiophene (EDOT), the oxidative reagent Fe(III)(OTf)<sub>3</sub>, and the polymerization rate controller PEG–PPG–PEG (average molecular weight ~14,600) in ethanol. The formulation with co-solvent was obtained by adding DMF or NMP to the aforementioned solution [1]. Preparation of precursor solution as well as deposition were carried out in nitrogen filled glovebox. The detailed procedure is presented as follows:

- 1) Preparation of solution A: absolute ethanol + PEG-PPG-PEG in the ratio of 80:20 % wt;
- 2) Preparation of solution A: Co-solvent (DMF or NMP) + PEG-PPG-PEG in the ratio of 80:20 % wt;
- 3) Mixing of solutions A and B in order to obtain the desired content of co-solvent in the final formulation;
- 4) Preparation of oxidative solution: Fe (III)(OTf)<sub>3</sub> is dissolved in mixed solution (A+B) to obtain concentration of 126 mg/ml;
- 5) Substrate cleaning: sonicate in CH<sub>2</sub>Cl<sub>2</sub> (3 minutes), sonicate in isopropanol (3 minutes), blow dry with N<sub>2</sub>;
- 6) Deposition: 0.25 mL of the oxidative solution is mixed (30s on vortex mixer) with 5 µL of EDOT before being spin coated on the clean substrate (1000 rpm/s, 4500 rpm, 30s). The substrate is then heated on a hot plate at 70°C for 15 minutes to accelerate polymerization before being rinsed with ethanol and blow dried with N<sub>2</sub>.

## 2. Calculation of cross-plane electrical conductivity

In order to calculate the cross-plane electrical conductivity of the film ( $\sigma_{film}$ ), we first calculate the contact area ( $A$ ) according to Hertz model of spherical indenter [2], given in the eq. (1).

$$A = \pi \left( \frac{r_{tip} F}{K} \right)^{\frac{2}{3}} \quad (1)$$

where  $r_{tip}$  is the tip radius (provided by Bruker),  $F$  is the applied force (N) and  $K$  is the reduced young modulus (N/m<sup>2</sup>) ( $1.4 \times 10^{10}$  N/m<sup>2</sup>, according to Cui *et al.* [2]). For example, we calculate  $A = 1.85 \times 10^{-17}$  m<sup>2</sup> from  $r_{tip} = 20$  nm and  $F = 10$  nN.

The electrical conductivity is calculated by using the eq. (2).

$$\sigma_{film} = \frac{d}{A R_{film}} \quad (2)$$

where  $d$  is the thickness of the film (m),  $A$  is the effective contact area (m<sup>2</sup>) and  $R_{film}$  ( $\Omega$ ) is the electrical resistance obtained from the linear fitting of I(V) data.

### 3. Lateral resolution of Scanning Thermal Microscopy (SThM) and calibration procedure for Null Point (NP) SThM quantitative measurements

When applying SThM for quantitative thermal analysis, it is important to understand its limitations, one of which is decreased lateral resolution (when compared to conventional AFM in contact mode). The surface of sample probed with SThM tip is higher due to inherently larger size of SThM probe as compared to conductive AFM (C-AFM), for example: tip curvature radius of 100nm for SThM tip VITA-HE-GLA-1 vs 25nm for C-AFM tip SCM PIC V2 from Bruker. This results to contact area radius of ~20nm (this estimation takes water meniscus into account, please see Section 10 of the Supplementary Information for the details) vs ~2.4nm (calculated from Hertz model in the Section 2). It is important to underline that the relatively large size of SThM probe comes from a tradeoff between the need to attain an acceptable level of thermal signal (the heat flow from the SThM tip is directly proportional to the tip/sample interface [3]) and the requirement of acceptable lateral resolution. The depth of the thermal analysis with SThM is estimated to be several times of the tip/sample contact radius [4]. Another thing to consider is the mechanical robustness of the tip and thin film Pd resistor (~45nm thickness) in its apex: decreasing the tip radius will most certainly imply a thinner Pd layer and negatively affect the lifetime of the probe. A viable strategy to increase the lateral thermal resolution of SThM would be to perform the measurements in UHV (or dry glovebox) conditions, since the thermal contact area will be decreased due to the absence of water meniscus. Work in UHV conditions will also allow to gain thermal conductivity resolution due to a decrease of thermal loss through the tip environment; i.e. more thermal power could be delivered to the sample, which would enable to accurately measure more thermally conductive materials (though it will decrease its sensitivity to samples presenting low thermal conductivity due to thermal contact area reduction).

To perform quantitative NP-SThM measurements, the heated SThM tip (temperature of the tip is controlled by the DC bias of the Wheatstone bridge) is brought in contact with the surface of the sample by performing a ramp in Z direction of the scanning probe microscope scanner. At the moment of contact, a rapid temperature change occurs due to induced heat flow from the heated tip into the sample. This temperature change is recorded as a voltage differential in the Wheatstone bridge of the SThM module, which allows us to obtain a sequence of temperature differential values for different probe temperatures.

We calculate the thermal conductivity  $\kappa$  by using the following relation [5]:

$$T_C - T_{amb} = \left[ \alpha \frac{1}{\kappa} + \beta \right] (T_{NC} - T_C) \quad (3)$$

where  $T_C$  is the probe tip temperature at contact, i.e. when the tip is in thermal equilibrium with the sample surface,  $T_{NC}$  is the tip temperature just before contact with the sample surface,  $T_{amb}$  is the ambient temperature, the calibration coefficients  $\alpha$  and  $\beta$  are related to thermal contact area, i.e. tip and sample geometry as well as tip-sample thermal conductance and parasitic heat flows [5].

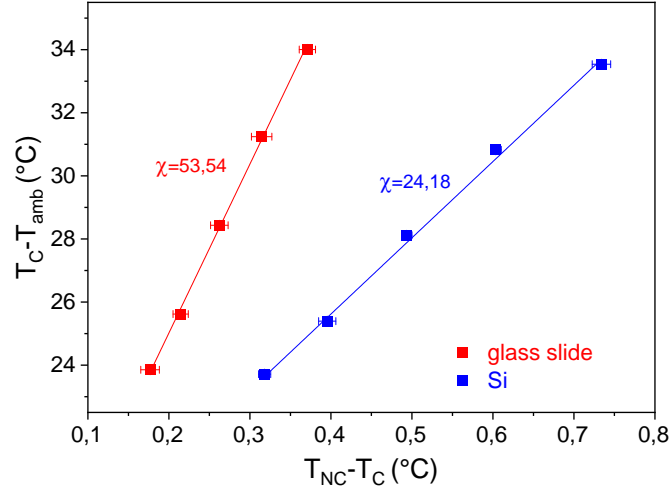

**Figure S1.** NP SThM calibration data for results presented in the Figure 4 in the main article.

The values of  $T_C - T_{amb}$  are plotted as a function of  $T_{NC} - T_C$  and we perform a linear fit of this plot to extract its slope,  $\chi$ , which is inversely proportional to the thermal conductivity. The thermal conductivity is obtained through prior calibration of the system using reference materials. For this purpose, reference materials are Si wafers (we assume its conductivity to  $148 \text{ Wm}^{-1}\text{K}^{-1}$ , with the native silicon oxide contribution being negligible [5]) and borosilicate microscope glass slide ( $\kappa = 1.3 \text{ Wm}^{-1}\text{K}^{-1}$ ). For example, the calibration values deduced from the measurements on the Si wafer and the glass slide in the Figure S1 are:  $\alpha = 7.49 \text{ Wm}^{-1}\text{K}^{-1}$  and  $\beta = 26.24 \text{ K K}^{-1}$ . These coefficients were further used to calculate  $\kappa$  of PEDOT:OTf film from the data presented in the Figure 4 of the main article. This calibration protocol is repeated to every tip used throughout this work since  $\alpha$  and  $\beta$  are tip-dependent.

#### 4. Topography of PEDOT:OTf thin films

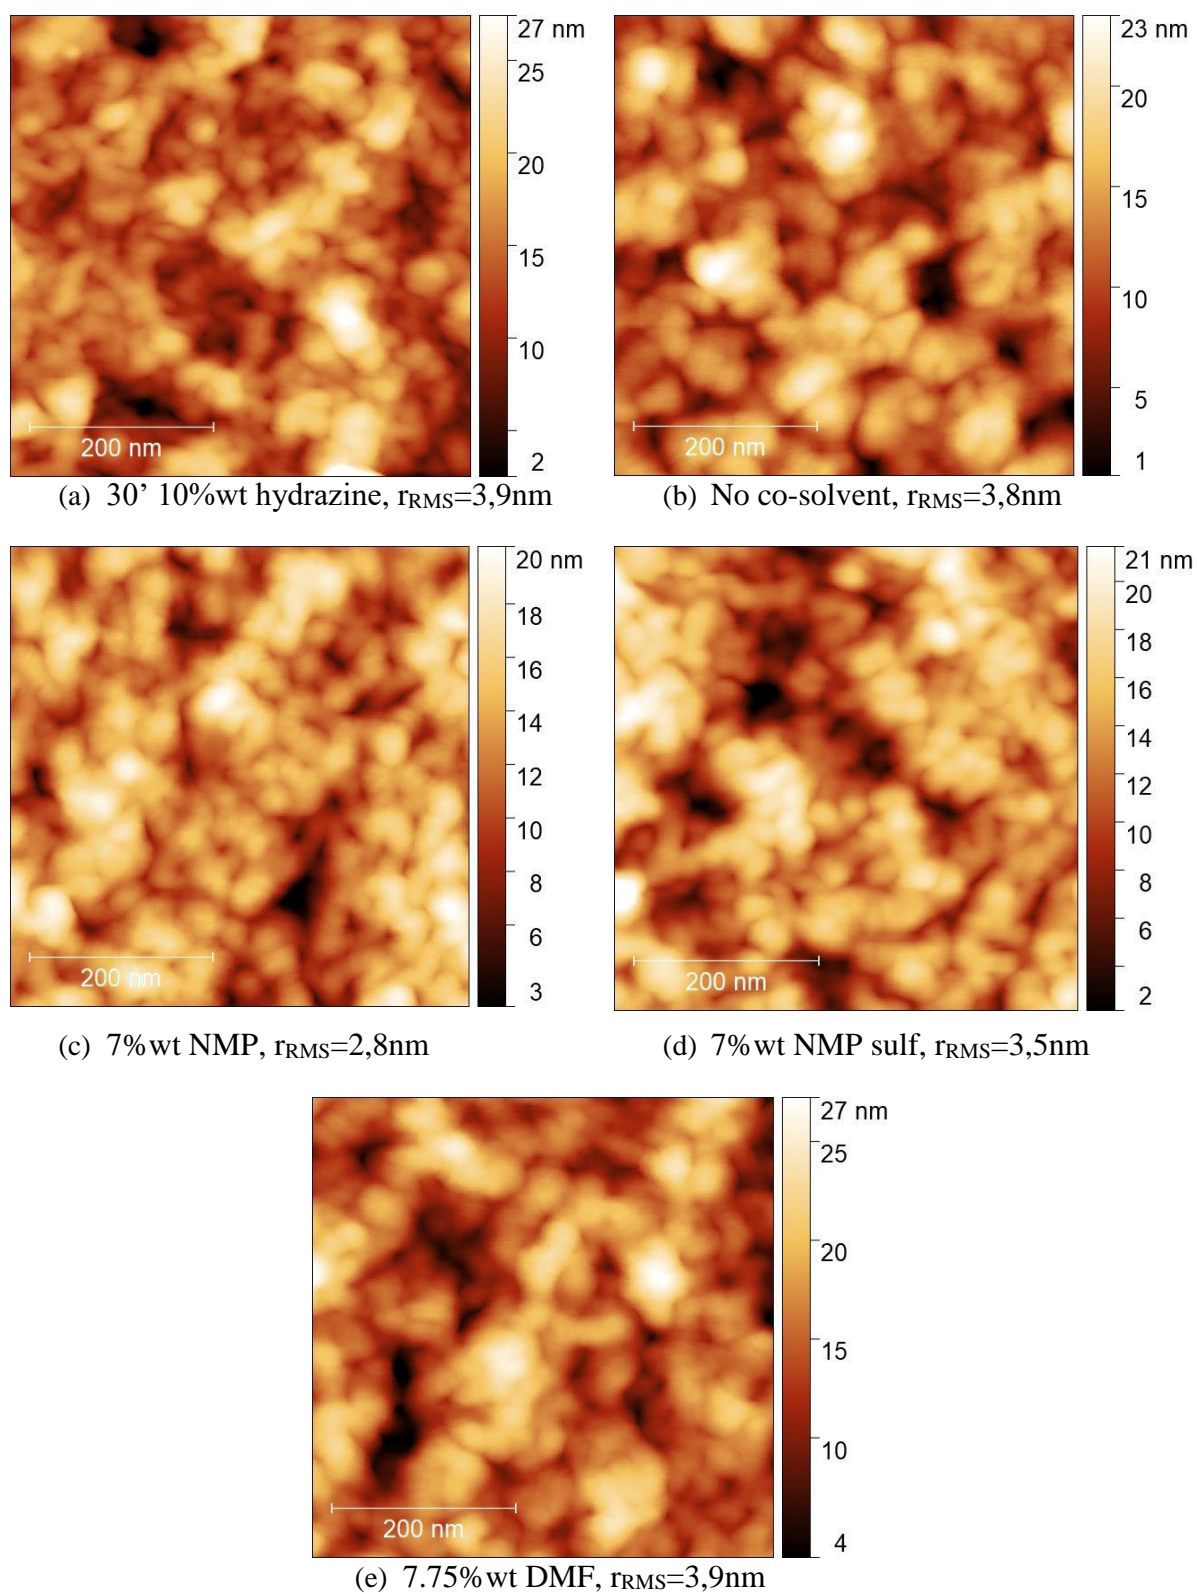

**Figure S2.** Topography of PEDOT:OTf thin films recorded with tapping mode AFM. Corresponding conditions and RMS roughness are indicated in the caption.

## 5. Thickness of PEDOT:OTf films

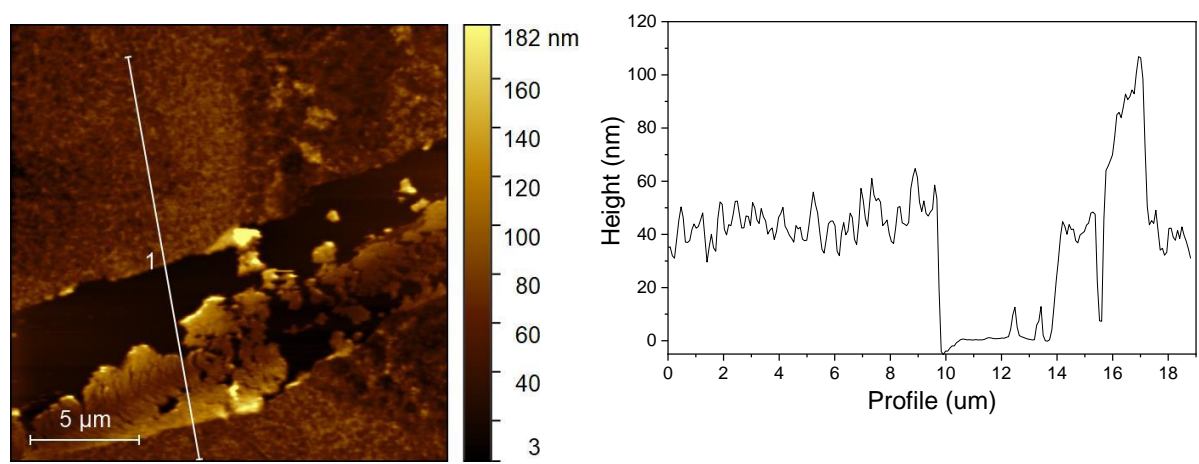

**Figure S3.** Topography of PEDOT:OTf thin film recorded with tapping mode AFM (left) after scratching with a sharp object. Profile (right) corresponding to the white line on the topography image.

## 6. Topography of the zone corresponding to the CAFM measurements

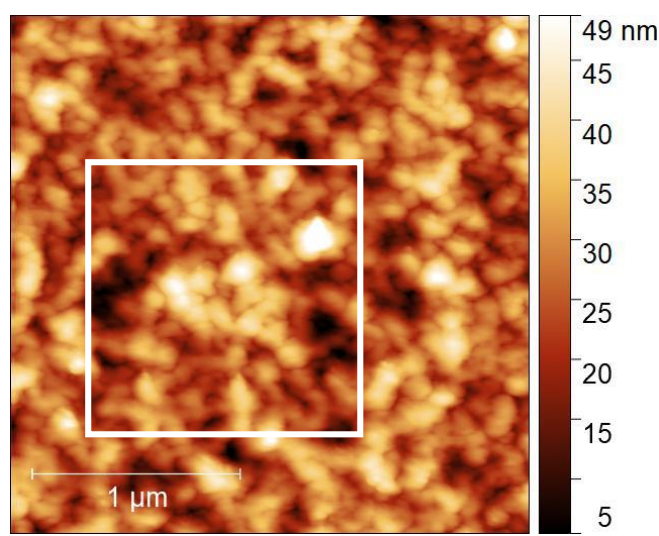

**Figure S4.** Topography of PEDOT:OTf thin film recorded with tapping mode AFM. White square corresponds to the C-AFM image area presented in the Figure 1 (a) and (b) of the main article.

## 7. In-plane electrical conductivity

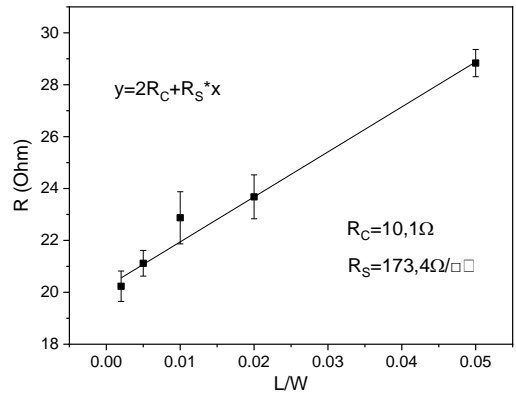

**Figure S5.** Transfer line measurements (TLM) of PEDOT:OTf film.

Measurements of in-plane electrical conductivity were carried out for a PEDOT:OTf film with no co-solvent for comparison with cross-plane data.

PEDOT:OTf film was deposited on a substrate with several electrode L/W ratios (Figure S5), the electrical resistance was measured with Agilent 4156C semiconductor analyzer in a glovebox.

Electrical conductivity  $\sigma$  was calculated with the following equation:

$$\sigma = \frac{1}{R_S \cdot d} \quad (4)$$

where  $R_S$  is the sheet resistance of the film deduced from the TLM plot and  $d$  is the film thickness. The in-plane electrical conductivity for pristine PEDOT:OTf was found to be  $1445 \pm 181$  S/cm ( $\pm 5$  nm film thickness variation).

## 8. Topography of the zone corresponding to the SThM images

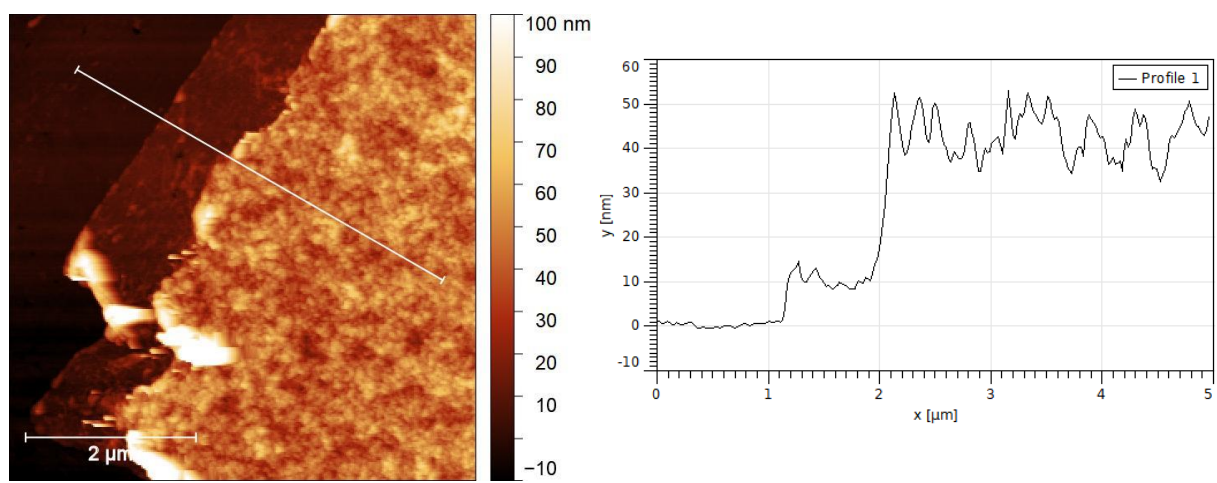

**Figure S6.** Topography (left) of PEDOT:OTf thin film recorded with tapping mode AFM corresponding to the area presented in the Figure 2 (a) and (b) of the main article. Profile (right) corresponding to the white line on the topography image.

## 9. Topography and Temperature profile

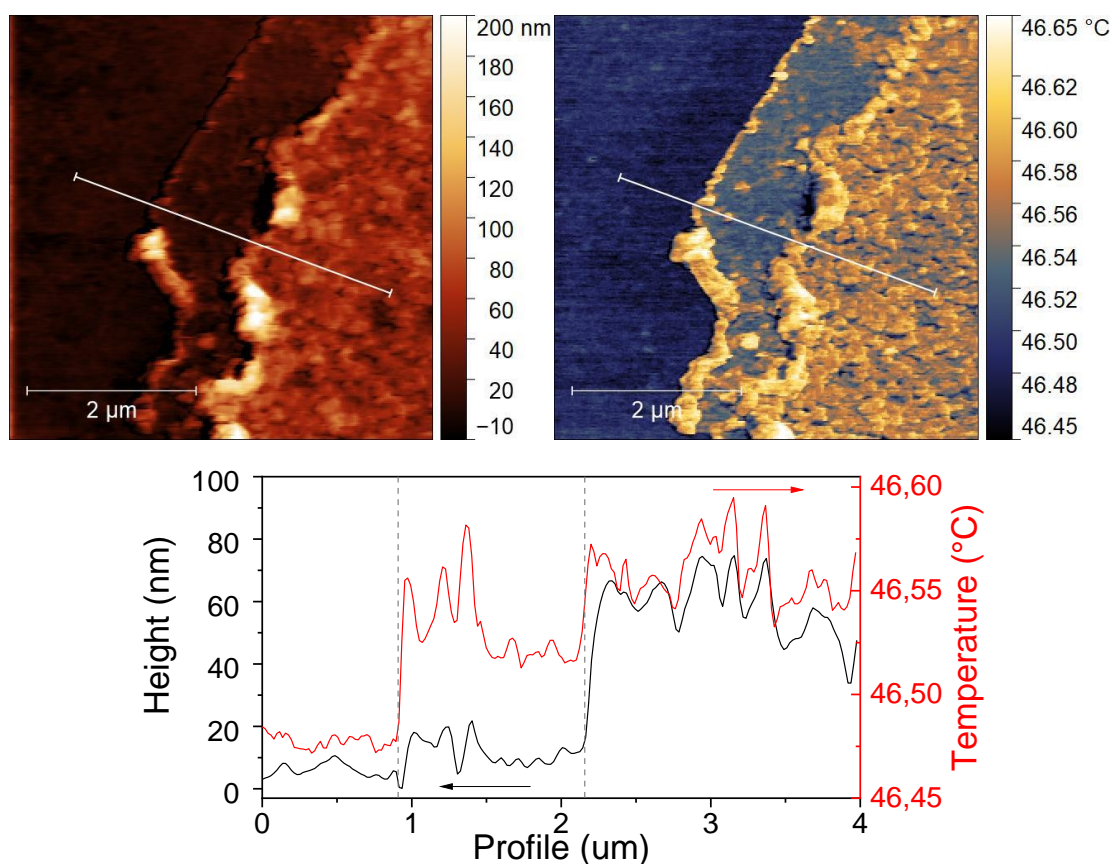

**Figure S7.** Topography (top left) and temperature mapping (top right) of PEDOT:OTf thin film presented in the Figure 2 (a) and (b) of the main article. Profile (bottom) corresponding to the white line on top two images.

## 10. Estimation of the radius of the thermal contact between the probe and the surface.

The thermal contact radius is calculated by following the procedure reported by Luo *et al* [6]. It takes into account the geometrical tip radius  $r_{tip}$  and the size of the water meniscus at the tip/surface interface. The thermal radius of the thermal contact is given by [7]:

$$r_{th} = 2.08 \sqrt{\frac{-r_{tip} \cos \theta}{\ln \varphi}} \quad (5)$$

where  $r_{tip} = 100$  nm (provided by Bruker), the relative humidity  $\varphi = 0.35$ -0.4 (air-conditioned laboratory) and the contact angle of the concave meniscus between the tip and the surface  $\theta \approx 30^\circ$  as reported for  $\pi$ -conjugated molecular crystals by Zhang *et al* [8]. The calculated thermal contact radius for our conditions is  $r_{th} \approx 20$  nm.

## 11. Calculation of PEDOT oxidation degree from the XPS measurements.

The oxidation degree of PEDOT:OTf is calculated from the integrated area (A) of S2p XPS signals of dopants and PEDOT from the following ratio:

$$\frac{A_{dopants}}{A_{thiophenes}} \times 100\% \quad (6)$$

**Table 1.** XPS data of PEDOT:OTf treated with H<sub>2</sub>SO<sub>4</sub> (oxidation degree 23.7%)

| Peak        | Thiophenes         |                    | Triflates          |                    | Sulfates           |                    |
|-------------|--------------------|--------------------|--------------------|--------------------|--------------------|--------------------|
|             | S2p <sub>3/2</sub> | S2p <sub>1/2</sub> | S2p <sub>3/2</sub> | S2p <sub>1/2</sub> | S2p <sub>3/2</sub> | S2p <sub>1/2</sub> |
| Energy (eV) | 163.70             | 164.86             | 168.19             | 169.35             | 168.58             | 169.74             |
| Area        | 1744               | 890                | 316                | 161                | 97                 | 49                 |

**Table 2.** XPS data of as-deposited PEDOT:OTf (oxidation degree 19.2%)

| Peak        | Thiophenes         |                    | Triflates          |                    |
|-------------|--------------------|--------------------|--------------------|--------------------|
|             | S2p <sub>3/2</sub> | S2p <sub>1/2</sub> | S2p <sub>3/2</sub> | S2p <sub>1/2</sub> |
| Energy (eV) | 163.71             | 164.87             | 167.96             | 169.12             |
| Area        | 1928               | 985                | 370                | 189                |

## 12. 2D I(V) histograms corresponding to the Figure 8 in the main article

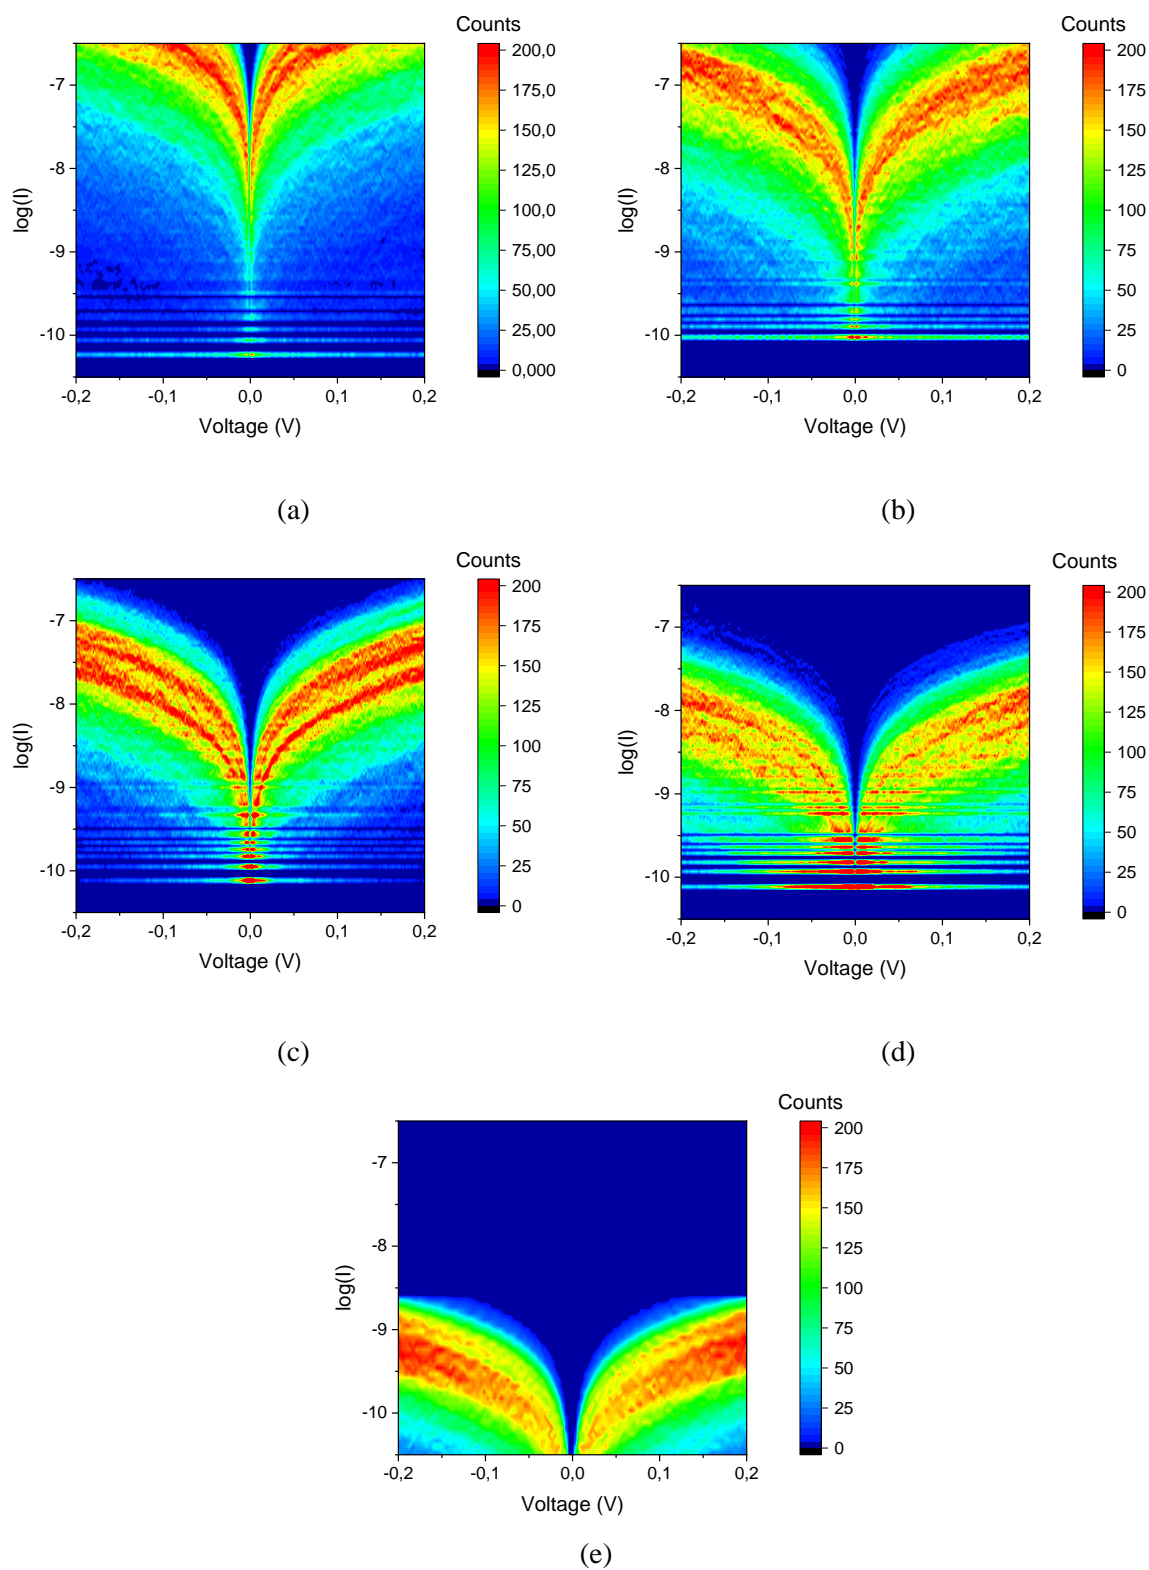

**Figure S8.** 2D I(V) histograms corresponding to the Figure 8 in the main article: (a) 7.75%wt DMF after  $H_2SO_4$  treatment,  $\log(R)=5.31\pm0.09$ , (b) no co-solvent,  $\log(R)=6.07\pm0.08$ , (c) 5' 10%wt  $NaBH_4$  solution treatment,  $\log(R)=6.95\pm0.08$ , (d) 10' of the same treatment,  $\log(R)=7.64\pm0.08$ , (e) 30' 10%wt hydrazine solution treatment,  $\log(R)=8.66\pm0.06$ .

### 13. NP SThM data

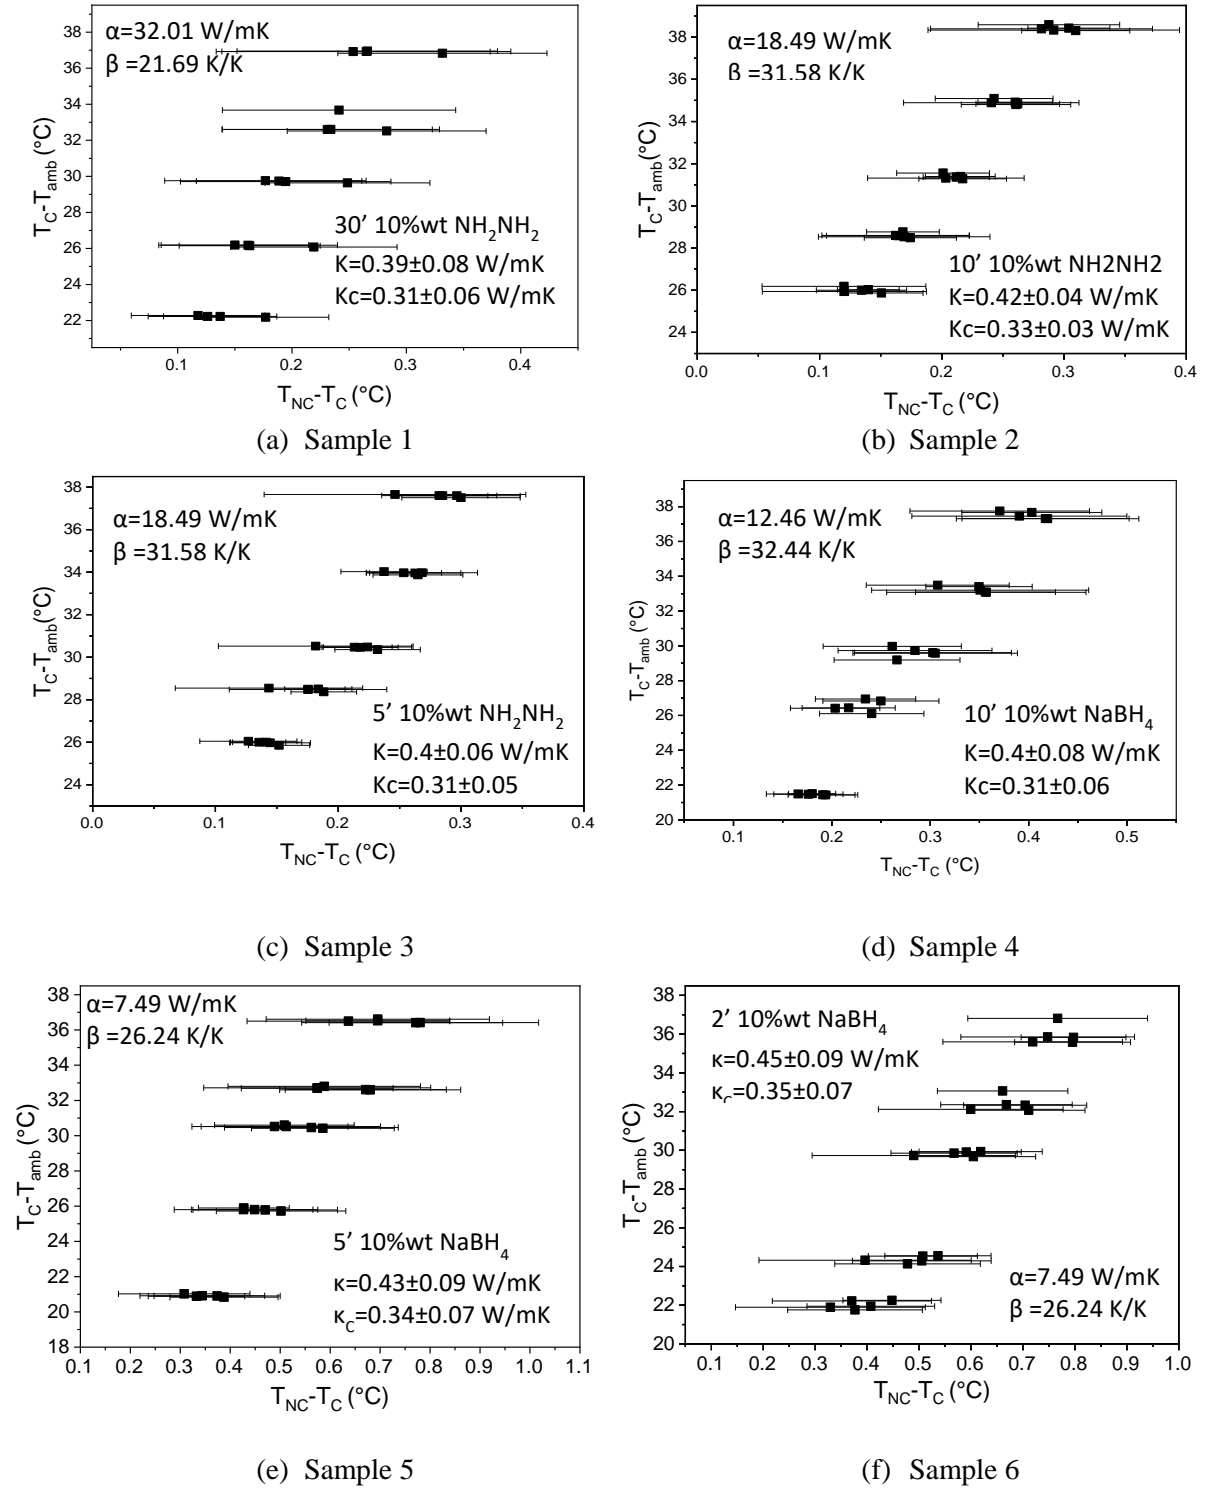

**Figure S9a.** NP-SThM data for PEDOT:OTf films after various treatments corresponding to the samples from 1 to 6 from Figure 9 in the main article. Treatment, thermal conductivity (before,  $\kappa$ , and after correction,  $\kappa_c$ ) as well as the calibration coefficients (depending on tip, see section S3) are presented in the legend.

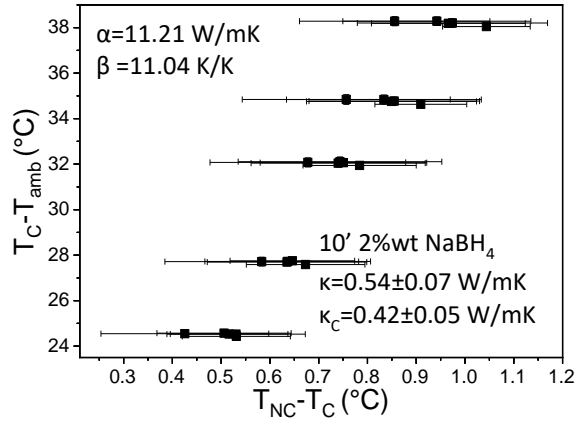

(g) Sample 7

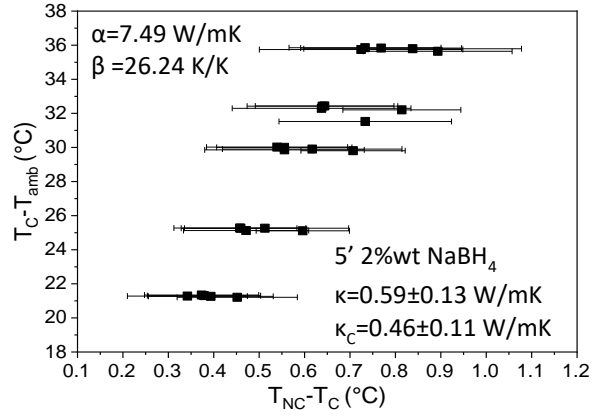

(h) Sample 8

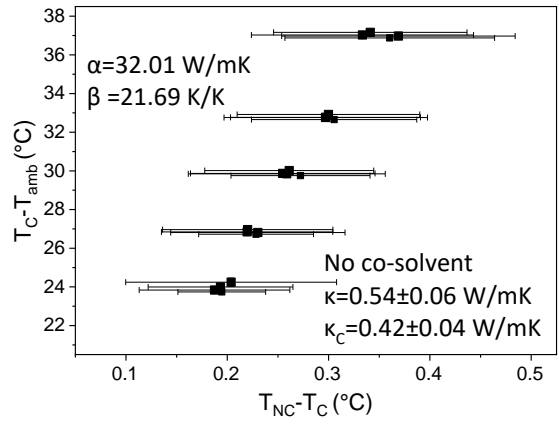

(i) Sample 9

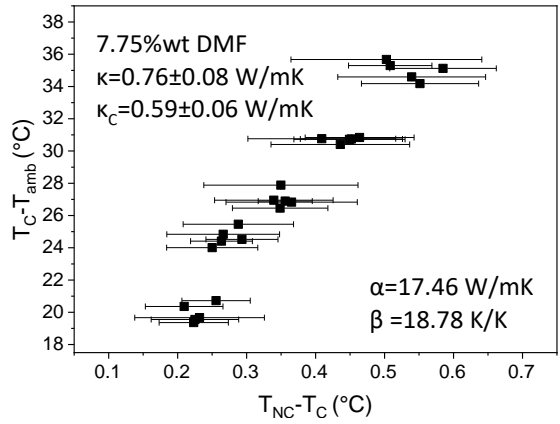

(j) Sample 10

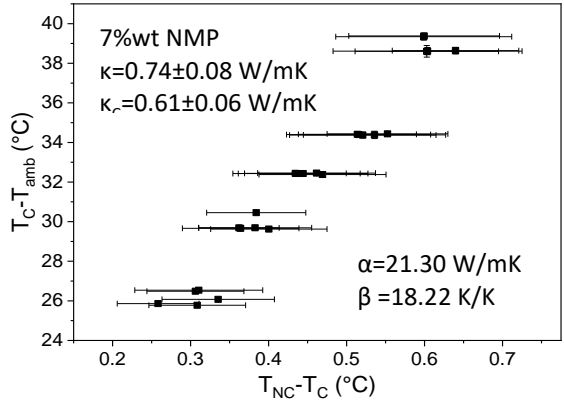

(k) Sample 11

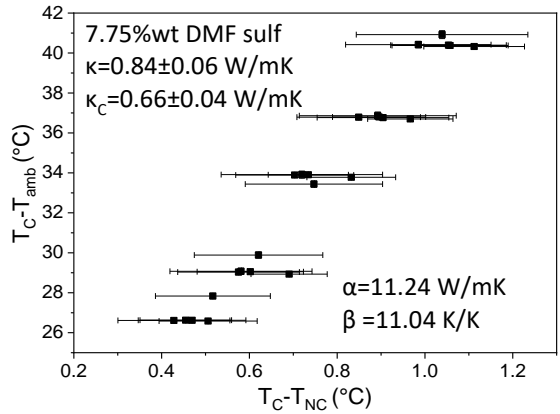

(l) Sample 12

**Figure S9b.** NP-SThM data for PEDOT:OTf films after various treatments corresponding to the samples from 7 to 12 from Figure 9 in the main article. Treatment, thermal conductivity (before,  $\kappa$ , and after correction,  $\kappa_c$ ) as well as the calibration coefficients (depending on tip, see section S3) are presented in the legend.

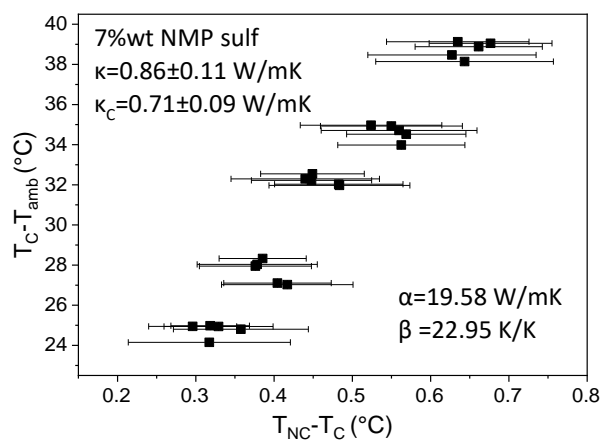

(m) Sample 13

**Figure S9c.** NP-SThM data for PEDOT:OTf films after various treatments corresponding to the sample 13 from Figure 9 in the main article. Treatment, thermal conductivity (before,  $\kappa$ , and after correction,  $\kappa_c$ ) as well as the calibration coefficients (depending on tip, see section S3) are presented in the legend.

## References

- [1] M. N. Gueye *et al.*, “Structure and Dopant Engineering in PEDOT Thin Films: Practical Tools for a Dramatic Conductivity Enhancement,” *Chem. Mater.*, vol. 28, no. 10, pp. 3462–3468, May 2016, doi: 10.1021/acs.chemmater.6b01035.
- [2] X. D. Cui *et al.*, “Making electrical contacts to molecular monolayers,” *Nanotechnology*, vol. 13, no. 1, pp. 5–14, 2002, doi: 10.1088/0957-4484/13/1/302.
- [3] Y. Zhang, W. Zhu, F. Hui, M. Lanza, T. Borca-Tasciuc, and M. Muñoz Rojo, “A Review on Principles and Applications of Scanning Thermal Microscopy (SThM),” *Adv. Funct. Mater.*, vol. 30, no. 18, p. 1900892, May 2020, doi: 10.1002/adfm.201900892.
- [4] S. Gomès, L. David, V. Lysenko, A. Descamps, T. Nychyporuk, and M. Raynaud, “Application of scanning thermal microscopy for thermal conductivity measurements on meso-porous silicon thin films,” *J. Phys. D. Appl. Phys.*, vol. 40, no. 21, pp. 6677–6683, 2007, doi: 10.1088/0022-3727/40/21/029.
- [5] K. Kim, J. Chung, G. Hwang, O. Kwon, and J. S. Lee, “Quantitative Measurement with Scanning Thermal Microscope by Preventing the Distortion Due to the Heat Transfer through the Air,” *ACS Nano*, vol. 5, no. 11, pp. 8700–8709, Nov. 2011, doi: 10.1021/nn2026325.
- [6] K. Luo, “Sensor nanofabrication, performance, and conduction mechanisms in scanning thermal microscopy,” *J. Vac. Sci. Technol. B Microelectron. Nanom. Struct.*, vol. 15, no. 2, p. 349, Mar. 1997, doi: 10.1116/1.589319.
- [7] J. N. Israelachvili, *Intermolecular and Surface Forces*. Elsevier, 2011.
- [8] Y. Zhang, C. Zhang, D. Wei, X. Bai, and X. Xu, “Nanoscale thermal mapping of few-layer organic crystals,” *CrystEngComm*, vol. 21, no. 36, pp. 5402–5409, 2019, doi: 10.1039/c9ce00827f.
